# Supplementary material for: Unified Questioner Transformer for Descriptive Question Generation in Goal-Oriented Visual Dialogue
Source: arXiv:2106.15550 source file (2021-06-29)
Supplement: Supplementary file 1 [file appendix.tex]

\section*{Appendix}
\noindent

\subsection{UniQer Model Details}
\nibf{Object Targeting Module (\S\redrb{4.3}).}
We show an overview of the Object Targeting Module (OTM)
with an example when $k=3$ in Fig.~\ref{fig:otm}.
The OTM groups objects $\mathcal{O}$ into three groups:
the target object group $\mathcal{O}_{\mathrm{t}}$,
the distracter object group $\mathcal{O}_{\mathrm{d}}$,
and the masked object group $\mathcal{O}_{\mathrm{m}}$.
Examples of the object groups and the corresponding questions are shown in Fig.~\ref{fig:property}.

\subsection{Evaluation Metrics}
\nibf{Perfect Address and Correct Address (\S\redrb{6.2}).}
Given a question $q$ and an answer $a$ from the \oracle{}, $\mathcal{O}$
will be divided into two object groups in mutually exclusive and collectively exhaustive manner:
a matched group $\mathcal{O}_{q}$ for objects that matches $(q, a)$
and an unmatched group $\overline{\mathcal{O}}_{q}$ otherwise.
In order for a question to be perfect or correct,
the target objects $\mathcal{O}_{\mathrm{t}}$ and
the distracter objects $\mathcal{O}_{\mathrm{d}}$
must be separately belongs to matched or unmatched group,
\ie{}, it must fulfill either
$\mathcal{O}_{\mathrm{t}} \in \mathcal{O}_{q} \wedge \mathcal{O}_{\mathrm{d}} \in \overline{\mathcal{O}}_{q}$ 
or
$\mathcal{O}_{\mathrm{t}} \in \overline{\mathcal{O}}_{q} \wedge \mathcal{O}_{\mathrm{d}} \in \mathcal{O}_{q}$.
What makes the difference between perfect and correct is whether
the masked objects are mixed with the target objects.
That is, when the target objects belong to the matched group
$\mathcal{O}_{\mathrm{t}} \in \mathcal{O}_{q}$,
the case $\mathcal{O}_{q} \bigcap \mathcal{O}_{m} = \{\phi\}$ is perfect
and, otherwise, correct.
Fig.~\ref{fig:property} also gives examples of 
perfect questions (\textit{ex.1} and \textit{ex.4})
and correct questions(\textit{ex.2} and \textit{ex.3}).
In \textit{ex.3}, objects are grouped as
$\mathcal{O}_t = \{\mathrm{green\_cylinder}\}$,
$\mathcal{O}_d = \{\mathrm{green\_sphere}\}$, and
$\mathcal{O}_m = \{\mathrm{red\_cylinder}\}$.
The question in \textit{ex.3} is correct, since it will divide the objects as
$\mathcal{O}_q = \{\mathrm{green\_cylinder, red\_cylinder}\}$ and
$\overline{\mathcal{O}}_q = \{\mathrm{green\_sphere}\}$,
while in \textit{ex.4} is perfect,
since the question addresses to the target objects without including the masked object as
$\mathcal{O}_q = \{\mathrm{green\_cylinder}\}$ and
$\overline{\mathcal{O}}_q = \{\mathrm{green\_sphere, red\_cylinder}\}$.

\subsection{Learning Details}
\nibf{Policy Gradient Optimization (\S\redrb{5.2}).}
In accordance with the existing studies, we adopt the policy gradient method~\cite{sutton2000policy}
for optimizing the \otgt{}.
% Computations of policy gradient optimization
The objective function will be
\begin{equation}
  J(\theta) = \mathbb{E}_{\pi_\theta}\left[\sum_{t=1}^{T}r(S_t, A_t)\right],
  \label{eq_pg}
\end{equation}
where $\pi_\theta$ represents the policy function parameterized with $\theta$.

Since policy gradient approach has a good convergence on high-dimensional action space,
it is suitable for our purposes.
The goal of policy gradient is to find the policy parameter $\theta$ that gives better expected rewards via gradient ascent.
With the episodic settings, the \questioner{} engages in multiple trajectories with length $T$
defined as $\tau = (S_0, A_0, R_0, \ldots, S_{T-1}, A_{T-1}, R_{T-1}, R_{T})$.
Given the trajectories, the gradients of the objective function will be approximated
by introducing \textbf{REINFORCE} algorithm~\cite{williams1992simple} as follows
\begin{equation}
  \nabla_{\theta} J(\theta) \approx \mathbb{E}_{\pi_\theta}\left[\sum_{t=0}^{T-1}\nabla_{\theta}\ln\pi_{\theta}(A_t|S_t)(G(t)-b(S_t))\right]
\end{equation}
where $G(t) = \sum_{t'=t}^{T-1}\gamma^{T-(t'+1)} R_{t'+1}$ is the return function with discount factor $\gamma$ applied.

\begin{figure}[tbp] \begin{center}
  \includegraphics[width=\linewidth]{./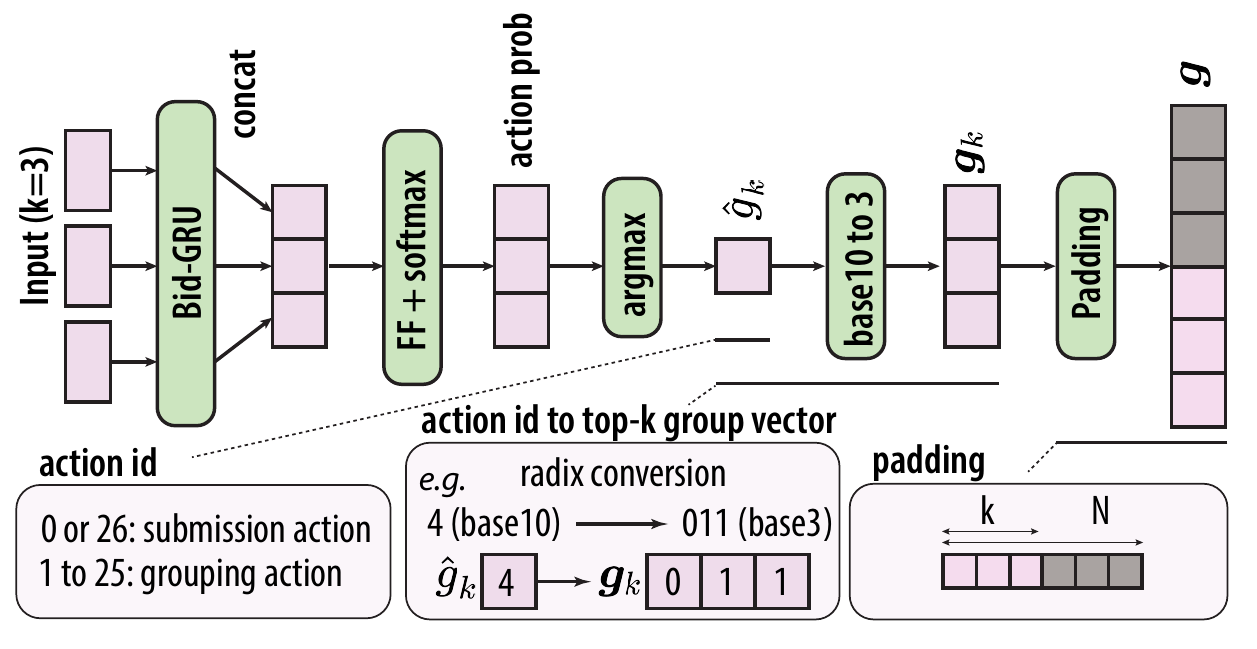}
  	\caption{
  	Overview of the Object Targeting Module (OTM).
  	In this figure, an example process of when $k=3$ and $N=6$ is demonstrated.
  	The input of the bidirectional GRU is
  	the object features in order of decreasing confidence.
    }
    \label{fig:otm}
  \end{center}
\vspace{-5mm}
\end{figure}
\begin{figure}[tbp] \begin{center}
  \includegraphics[width=\linewidth]{./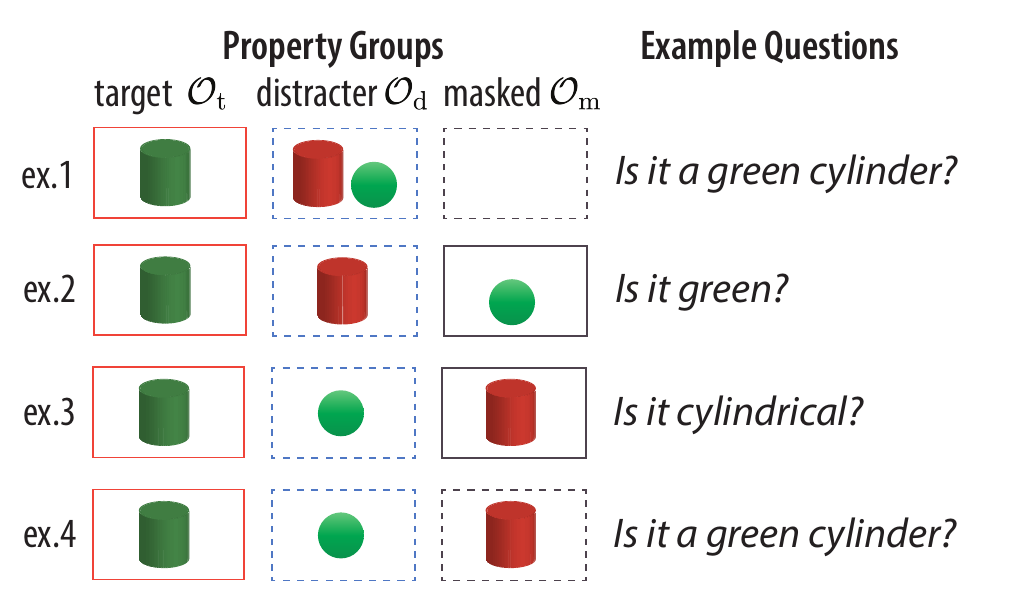}
  	\caption{
  	Example of possible questions given objects with three property groups;
    the target object group $\mathcal{O}_{\mathrm{t}}$,
    the distracter object group $\mathcal{O}_{\mathrm{d}}$,
    and the masked object group $\mathcal{O}_{\mathrm{m}}$.
    Given such object groups from the OTM, the QDT is required to
    generate questions that discriminate target objects from distracter objects.
  	Groups with solid line represent matched objects
  	if an answer to a question is \textit{yes}
  	and groups with dotted lines represent unmatched objects.
    Here, \textit{ex.1} and \textit{ex.4} are the perfect questions,
    and \textit{ex.2} and \textit{ex.3} are the correct questions.
    }
    \label{fig:property}
  \end{center}
\vspace{-5mm}
\end{figure}
\begin{algorithm}[t]
% \setstretch{1.2}
\SetAlgoLined
\SetKwIF{If}{ElseIf}{Else}{if}{:}{elif}{else:}{end}
{\footnotesize
\LinesNumbered
\KwData{$\mathcal{O}$}
% \KwResult{$G’=(X,V)$ with $V\subseteq U$ such that $G’^{tc}$ is an interval order.}
% $\triangleright$ initialization \\
% loop for one scene
The Oracle picks an goal object $o^{*} \in \mathcal{O}$ \\
q = [], a = []  \hfill $\triangleright$ questions $\&$ answers \\
\For(\hfill $\triangleright$ dialogue loop){$t=1$ \KwTo $T$}{
    $\triangleright$ Prepare embeddings  \hfill $\triangleright$ see \S\redr{4.1}\\
    $\bm{x}_{v} \leftarrow \mathcal{F}_{v}([\bm{o}_{v}(i), \bm{o}_g^{\mathcal{N}}(i)]_{i\in \mathcal{N}})$\\
    $\bm{x}_{l}^{t} \leftarrow{} [\mathrm{[CLS]}, w_1^1, w_2^1,..., w_{W_1}^1, a^1, w_1^{2}, ..., a^{t-1}]$ \\
    $\bm{x}_{h} \leftarrow [\bm{x}_{v}, \bm{x}_{l}^{t}]$  \\
    $\bm{x}_{e} \leftarrow \bm{x}_{h} + \bm{x}_{\mathrm{seg}} + \bm{x}_{\mathrm{pos}}$  \\

    $\triangleright$ \oet{} \hfill $\triangleright$ see \S\redr{4.2}\\
    $\{\tilde{\mathcal{X}}_{o}, \tilde{X}_{[\rm CLS]}, \tilde{\mathcal{X}}_{l}\} \leftarrow \oet{}(\bm{x}_{e})$ \\
    $\sigma_{o} \leftarrow [\mathrm{sigmoid}(\mathcal{F}_{o}(\tilde{X}_{o}^{i}) \cdot \mathcal{F}_{c}(\tilde{X}_{[\rm CLS]}))]_{i \in\mathcal{N}}$\\
    ${P}_{\hat{o}} \leftarrow \mathrm{softmax}(\sigma_o)$\\

    % OTM
    $\triangleright$ \otgt{} \hfill $\triangleright$ see \S\redr{4.3}\\
    Get top-k object ids: $\mathcal{K} \leftarrow \mathrm{argtopk}({P}_{\hat{o}})$ \\
    % prepare top-k features
    % $\bm{x}_{k} = [\bm{o}_{v}(i), \bm{o}_{g}(i), \bm{o}_{g}(i, j), {P}_{\hat{o}}(i)]_{(i, j) \in \mathcal{K}}$ \\
    $\bm{x}_{k} \leftarrow [\mathcal{F}_{A}(\bm{o}_{v}(i)), \mathcal{F}_{B}(\bm{o}_{g}^{\mathcal{K}}(i)), \mathcal{F}_{C}({P}_{\hat{o}}(i))]_{i \in \mathcal{K}})$ \\
    % $\bm{\hat{g}}_k \leftarrow \mathrm{softmax}(\mathcal{F}_{l}(\mathrm{concat}[\mathcal{F}_{\mathrm{GRU}}(\bm{x}_{k})]))$ \\
    $A_t \leftarrow \mathrm{sampling}(\mathcal{F}_{\mathrm{RL}}(\bm{x}_{k}))$\\
    % $\bm{\hat{g}_k}_{base3} = \mathrm{ternary}(\mathrm{argmax}(\bm{\hat{g}_k})) \hfill \triangleright~\text{size k}$\\
    $\bm{g}_{k} \leftarrow \mathrm{ternary}(A_{t}) \hfill \triangleright~\bm{g}_k \in \mathbb{R}^{3 \times k}$\\
    $\bm{g} \leftarrow \mathrm{padding}(\bm{{g}}_{k}) \hfill \triangleright~\bm{g} \in \mathbb{R}^{3 \times \mathcal{N}}$ \\

    \uIf({\hfill $\triangleright$ end of dialogue (EOD)})
    {$A_t \in \{0, 3^{k} - 1\}$}{
        $r(S_t, A_t) \leftarrow
        \begin{cases}
            1 - r_{d}(t) & \text{if}~\mathrm{argmax}(P_{\hat{o}})==o^{*}_{id} \\
            0 & \text{otherwise}
        \end{cases}
        $\\
        break
    }
    \uElseIf({\hfill $\triangleright$ EOD should have been generated}){$t == T$}{
        % if <EOD> is not generated --> cannot acquire rewards
        $r(S_t, A_t) \leftarrow 0$\\
    }
    \Else{
        $\triangleright$ \qdt{} \hfill $\triangleright$ see \S\redr{4.4}\\
        $\mathcal{M} \leftarrow \tilde{\mathcal{X}}_{o} + \mathcal{F}_{s}(\bm{g})$ \\
        $[w_1^t, w_2^t, ..., w_{W_t}^t] \leftarrow \mathrm{\qdt{}}(\mathrm{[BOS]}, \mathcal{M})$ \\
        append $[w_1^t, w_2^t, ..., w_{W_t}^t]$~to~q, ~$a^t$~to~a \\
    }
}
\caption{\propmodel{} RL flow for a scene}
\label{alg:Algo}
}
\end{algorithm}

\nibf{Implementation Details (\S\redrb{6.1}).}
\propmodel{} was implemented in PyTorch
and the \oracle{} was implemented using the engine proposed by \cite{johnson2017clevr}. 
All experiments were conducted using six Quadro RTX 8000 GPUs.
The parameter setting for the encoder and the decoder was:
d\_model=512, n\_head=8, dim\_feedforward=512, n\_layers=3, and dropout=0.1.
As an image feature extractor, we used Imagenet pre-trained ResNet34~\cite{he2016deep}.
It took approximately two days for \propmodel{} to train from scratch on a single GPU.

\nibf{Turn Discount Factor \boldmath{$r_d$} (\S\redrb{6.3}).}
The turn discount factor $r_d$, which reduces the reward based on the number of questions, 
is introduced to promote a more efficient questioning strategy
by trying to minimize the number of questions.
Without this discount factor, 
the agent tends to repeat the same question it  already asked during the dialogue even after it finds the correct goal object. 
We define the turn discount factor $r_d$ as:
\begin{align}
    r_d(t) = \beta * \cfrac{t}{T}~,
\end{align}
where $\beta$ is a coefficient that determines the scale of the penalty,
$t$ is the number of generated questions,
and $T$ is the maximum number of questions allowed for the agent.
Our experiments were conducted with $\beta=0.2$ and $T=5$.
Just to be sure, the agent should generate a special token, end of dialogue~(EOD),
to receive a reward before the number of questions reaches $T$.
Therefore our final reward function is described as:
\begin{equation}
    r(S_t, A_t) = 
    \begin{cases}
        1 - r_d(t) & \text{if}~\mathrm{argmax}(P_{\hat{o}})==o^{*}_{id} \\
        0 & \text{otherwise}
    \end{cases}.
\end{equation}

\nibf{RL algorithm (\S\redrb{5.2}).}
The overall procedure of reinforcement learning is shown in Algorithm~\textcolor{red}{1}.
The detailed explanation of each equation is denoted in the corresponding section.

\subsection{Baseline Model Details (\S\redrb{6})}
% What is the component of the Questioner?
In a manner similar to that of the previous studies~\cite{de2017guesswhat,strub2017end},
we divide the role of the questioner into the following four components:
\begin{itemize}
    \item \textbf{Question and Answer Encoder (QAE)}: An LSTM module encoding the current quesion and the answer given by the \oracle{}.
    \item \textbf{Dialogue State Encoder (DSE)}: An LSTM module encoding past dialogues.
    \item \textbf{Question Generator (QGen)}:
    An LSTM module generating a question based on the DSE's output and the top-k object features with high $P_{\hat{o}}$.
    \item \textbf{Guesser}: An MLP module for outputting candidate probabilities
    $P_{\hat{o}}$ using the features of an object as the input.
\end{itemize}
% Two steps of training
The Guesser, accompanied by the QAE and the DSE, and the QGen
are trained separately in the upstream tasks in a supervised manner,
and then merged into a single agent model to conduct reinforcement learning.

\nibf{Question and Answer Encoder (QAE)}
The QAE encodes the question tokens generated
by the QGen and the corresponding answer
provided by the Guesser. The encoded features will be passed to the DSE.
This function is implemented by a standard LSTM.

\nibf{Dialogue State Encoder (DSE)}
The DSE generates a dialogue state vector
$\tilde{X}_{\mathcal{D}}$ that holds the history of questions and answers.
$\tilde{X}_{\mathcal{D}}$ is used to both generate the next question token
in the QGen and compute the goal object probabilities $P{\hat{o}}$ in the Guesser.
This function is implemented by a standard LSTM.

\nibf{Question Generator (QGen)}
Formally, the QGen can be thought of as the probabilistic language model,
which sequentially generates a word $w_l^t$ to compose a question $q^t$,
given the previous word token $w_{l-1}^t$,
the dialogue history vector $\tilde{X}_{\mathcal{D}}$,
the context image feature $\bm{x}'_v$ extracted by the image feature extractor
and tok-k object feature embedding $\bm{x}_k$.
This can be formalized as follows:
\begin{align}
  P(w_{l+1}^t|w_{l}^t, \tilde{X}_{\mathcal{D}}, \bm{x}'_v, \bm{x}_k).
\end{align}
We employed the LSTM to implement such functions.

\nibf{Guesser}
The Guesser guesses the goal object $o^*$ based
on the current scene and the question answer history as:
\begin{align}
  P(\hat{o}^{*}|\bm{x}_v, \tilde{X}_{\mathcal{D}}).
\end{align}
We implement this function as:
\begin{align}
    P_{\hat{o}} = \mathrm{softmax}(
    [\mathrm{sigmoid}(\mathcal{F}_1(\bm{x}_v^i)\cdot
    \mathcal{F}_2(\tilde{X}_{\mathcal{D}}))]_{i \in \mathcal{N}}),
\end{align}
where $\mathcal{F}_1$ and $\mathcal{F}_2$ are the linear transformation functions.
While this operation is similar to Eqs.~(\redr{3}, \redr{4}),
the other object features are not compared when computing a probability for an object.

\nibf{Supervised Learning}
% What is the loss function of the network?
The loss function of the Guesser is as same as the
object prediction loss defined in Eq.~(\redr{8}),
where the QAE and the DSE will be jointly trained.

The loss function of the QGen is described as:
\begin{align}
  L_{\mathrm{gen}} = -\sum_{t=1}^{T}\sum_{l=1}^{W_t}
  \log p(w_{l+1}^t|w_{l}^t, \bm{h}),
\end{align}
where $\bm{h}$ is the hidden vector of the model,
$T$ is the maximum number of questions in a dialogue, and
$W_t$ is the number of tokens included in the $t$-th question.

\nibf{Reinforcement Learning}
Since the baseline model produces a word token on each iterative step,
the global timestep for the baseline model $t'$ is defined as
$t'=\sum_{\tau=1}^{t-1} |\mathcal{D}_\tau| + l$,
where $|\mathcal{D}_\tau|$ is the length of a past dialogue and $l$ is the step in the current dialogue.
% What are the actions in this game?
The set of actions $A_{t'}$ corresponds to the tokens in the vocabulary $\mathcal{V}$.
% What are the states in this game?
The state is defined as follows:
\begin{equation}
  S_{t'} = (\mathcal{I}, {(q^\tau, a^\tau)}_{1:t-1}, (w_1^t, \ldots, w_l^t)).
\end{equation}
The transition to the next state depends on the selected action:
\begin{itemize}
  \item If $A_{t'+1} = \textrm{\token{EOD}}$, the dialogue terminates.
  Thus, $S_{t'+1}$ becomes the last state.
  \item If $A_{t'+1} = \textrm{\token{EOS}}$, the current question generation terminates and
    the \questioner{} receives an answer $a^{t}$.
    The next state will be $S_{t'+1} = (\mathcal{I}, {(q^\tau, a^\tau)}_{1:t})$.
  \item Otherwise, if the generation of the question continues,
    the next state will be
    $S_{t'+1} = (\mathcal{I}, {(q^\tau, a^\tau)}_{1:t-1}, (w_1^t, \ldots, w_l^t, w_{l+1}^t))$
\end{itemize}

The model will be trained with
policy gradient optimization as introduced in Eq.~(\ref{eq_pg}).

\subsection{Supplementary Results (\S\redrb{6})}
\nibf{Average Vocabulary of Questions (\S\redrb{6.3}).}
Since our CLEVR Ask task comprises images that include multiple identical objects,
descriptive questions are a requirement for task success by nature.
Therefore, the descriptiveness of the questions can be evaluated by
how well the model performed in such an environment (\ie{} the task success ratio).

The descriptiveness can be also measured as the number of a question's unique attributes,
such as colors, sizes, and spatial relations. % , used in a single question.
We therefore introduced two metrics: $n_{\mathrm{vocab}}$, which shows the average vocabulary size of the questions, and $\overline{n}_{\mathrm{vocab}}$, which shows the average vocabulary size of the dialogues. They are defined as
\begin{align}
    n_{\mathrm{vocab}} &= \frac{1}{N_{\mathrm{data}}}\sum_{\mathcal{D} \in \mathrm{data}}{} \frac{1}{T_{\mathcal{D}}}
    \sum_{t=1}^{T_{\mathcal{D}}}
    |\{w_{\omega}^{t}\}_{\omega=1}^{W_t}|,\label{eq:vocab_question}\\
    \overline{n}_{\mathrm{vocab}} &= \frac{1}{N_{\mathrm{data}}}\sum_{\mathcal{D} \in \mathrm{data}}{} \frac{1}{T_{\mathcal{D}}}
    |\bigcap_{t=1}^{T_{\mathcal{D}}}
    \{w_{\omega}^{t}\}_{\omega=1}^{W_t}|
    ,\label{eq:vocab_dialogue}
\end{align}
where $N_\mathrm{data}$ is a number of data samples and
$T_{\mathcal{D}}$ is a number of questions in a dialogue $\mathcal{D}$.

\begin{table}[]
\footnotesize
\begin{centering}
 \begin{tabularx}{.47\textwidth}{@{}lcccc@{}}
 \toprule
                          & \multicolumn{2}{c}{Question Mean ($n_\mathrm{vocab}$)}
                          & \multicolumn{2}{c}{Dialogue Mean ($\overline{n}_\mathrm{vocab}$)} \\ \midrule
 Model & New Img   & New Obj  & New Img & New Obj \\ \midrule
 \multicolumn{1}{c}{Ask3} &                    &                  &                   &                  \\ \midrule
 Baseline   & $1.48_{ \pm 0.27 } $ & $1.48_{ \pm 0.27 }$   &    $3.15_{ \pm 0.08 } $ & $3.15_{ \pm 0.07 }$ \\
Ours(v)    & $2.62_{ \pm 0.04 } $ & $2.58_{ \pm 0.08 }$   &    $3.54_{ \pm 0.13 } $ & $3.54_{ \pm 0.16 }$ \\
Ours(num)  & $1.54_{ \pm 0.04 } $ & $1.52_{ \pm 0.03 }$   &    $2.92_{ \pm 0.11 } $ & $2.98_{ \pm 0.12 }$ \\
Ours(nu)   & $1.51_{ \pm 0.02 } $ & $1.47_{ \pm 0.07 }$   &    $3.11_{ \pm 0.17 } $ & $3.12_{ \pm 0.12 }$ \\
Ours(full) & $3.32_{ \pm 0.16 } $ & $3.35_{ \pm 0.08 }$   &    $3.82_{ \pm 0.12 } $ & $3.84_{ \pm 0.20 }$ \\
 \multicolumn{1}{c}{}     &                    &                  &                   &                  \\
 \multicolumn{1}{c}{Ask4} &                    &                  &                   &                  \\ \midrule
Baseline   & $1.00_{ \pm 0.00 } $ & $1.00_{ \pm 0.00 }$   &    $3.03_{ \pm 0.06 } $ & $3.05_{ \pm 0.03 }$ \\
Ours(v)    & $2.13_{ \pm 0.05 } $ & $2.10_{ \pm 0.04 }$   &    $3.44_{ \pm 0.24 } $ & $3.47_{ \pm 0.22 }$ \\
Ours(num)  & $1.56_{ \pm 0.03 } $ & $1.60_{ \pm 0.08 }$   &    $3.12_{ \pm 0.09 } $ & $3.09_{ \pm 0.05 }$ \\
Ours(nu)   & $1.56_{ \pm 0.04 } $ & $1.59_{ \pm 0.05 }$   &    $3.19_{ \pm 0.08 } $ & $3.13_{ \pm 0.06 }$ \\
Ours(full) & $1.49_{ \pm 0.02 } $ & $1.54_{ \pm 0.05 }$   &    $3.06_{ \pm 0.08 } $ & $3.06_{ \pm 0.04 }$ \\
 \bottomrule
 \end{tabularx}
  \caption{Question vocabulary for comparative models presented in Tab.~\redr{2}.
    Here, $n_{\mathrm{vocab}}$ shows the average vocabulary size of the questions,
    and $\overline{n}_{\mathrm{vocab}}$, which shows the average vocabulary size of the dialogues.
  % \txtodo{Add definitions of question mean and diglogue mean.}
}\label{tab:results_vocab}
\end{centering}
% \vspace{-1em}
\end{table}

Summarized results are shown in Tab.~\ref{tab:results_vocab}.
The question mean in Ask3 was 1.48 for \textit{Baseline} and 3.32 for \textit{Ours (full)},
while the dialogue mean was 3.15 for \textit{Baseline} and 3.84 for \textit{Ours (full)}.
The results indicate that, when asking a question, \propmodel{} uses
more than three attributes in its questions, \eg{} \textit{``Is it to the LEFT of a RED CUBE?''},
while the baseline asks trivial questions with a single attribute, \eg{} \textit{``Is it a SPHERE?''}
They also show that \propmodel{} has the richest vocabulary in a dialogue.
The results in Ask4 are less significant compared with Ask3,
while \propmodel{} still uses more than one attributes in a question.
The question mean and the dialogue mean were highest with \textit{Ours (v)} condition.
However, as shown by the task success ratio presented in Tab.~\redr{2},
the generated questions were not as effective as with \propmodel{}.

\begin{figure*}[tbp] \begin{center}
  \includegraphics[width=\linewidth]{./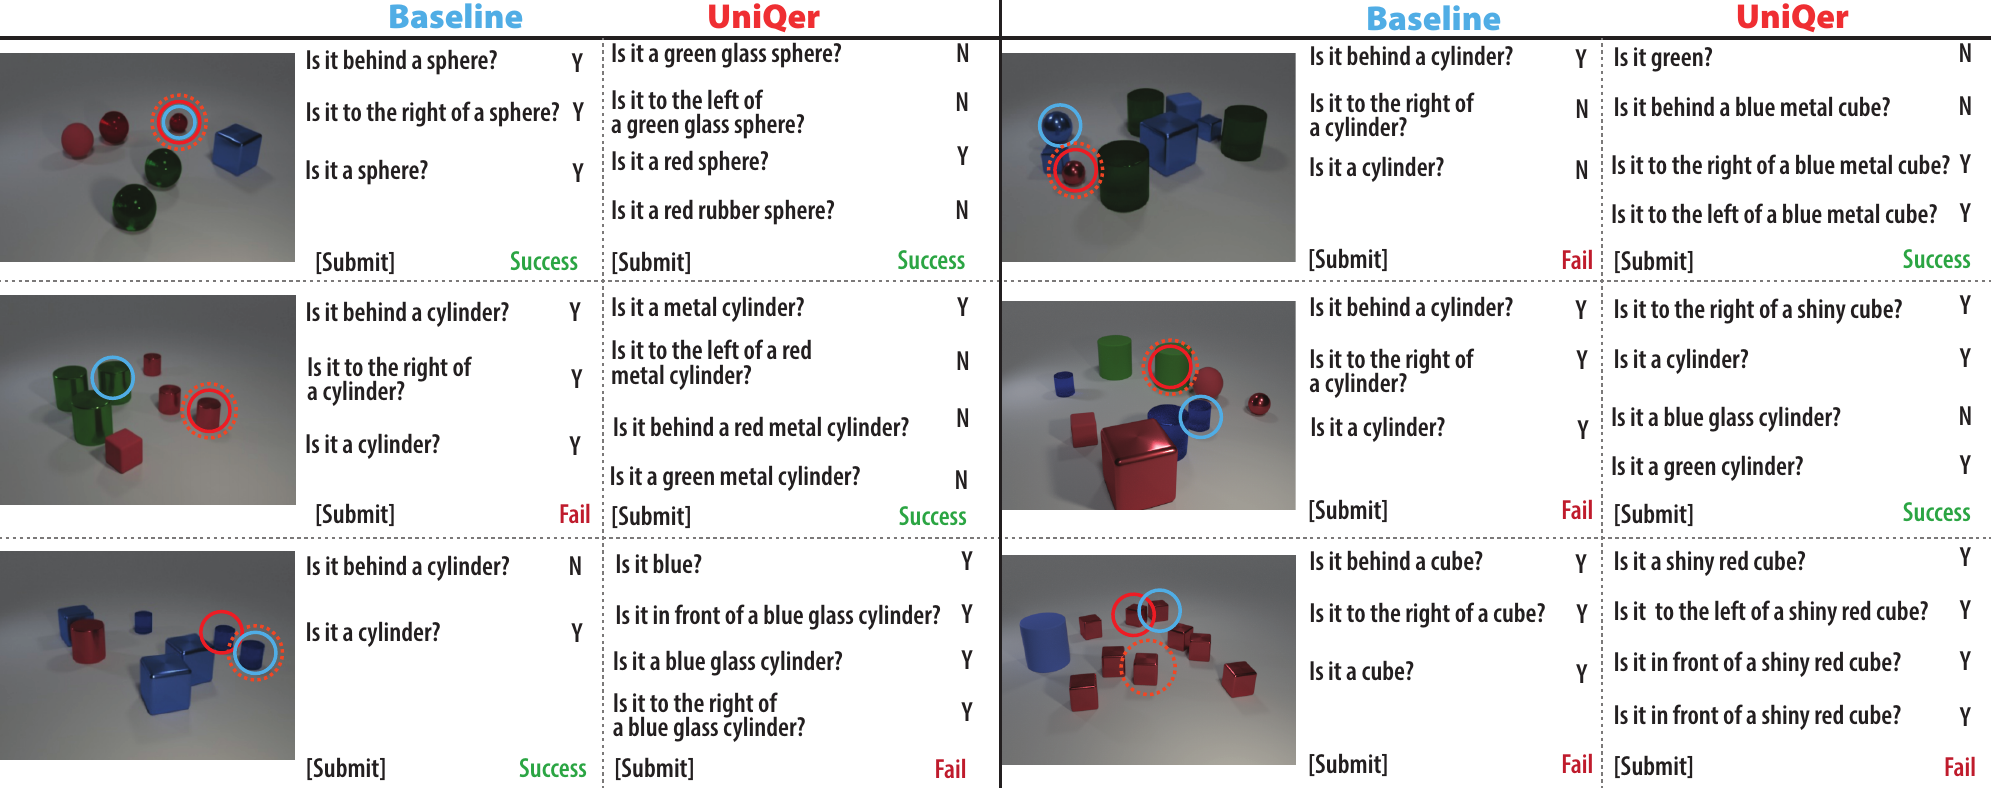}
  	\caption{
  	Additional qualitative samples from \textit{Baseline} and \propmodel{}.
    }
    \label{fig:appendix_samples}
  \end{center}
\vspace{-5mm}
\end{figure*}

\nibf{Stop Conditions (\S\redrb{6.3}).}
Additional results on the stop condition is presented in Tab.~\ref{tab:results_fs}.
The result shows that our model outperformed in the stop condition as well.
Compared with the results obtained without stop conditions, which were presented
in Tab.~\redr{2},
the variance for \propmodel{} decreased; however, there were no significant differences.
\begin{table}[]
\footnotesize
\begin{centering}
  \begin{tabularx}{.47\textwidth}{@{}p{1.45cm}p{1.3cm}p{1.3cm}p{1.3cm}p{1.3cm}@{}}
    \toprule
%                & \multicolumn{3}{c}{Task Success (\%)} \\ \midrule
    \multicolumn{1}{c}{} & \multicolumn{2}{c}{Ask3}                 & \multicolumn{2}{c}{Ask4}                                                      \\ \midrule
    Model                & New Img$\uparrow$ & New Obj$\uparrow$ & \multicolumn{1}{l}{New Img$\uparrow$} & \multicolumn{1}{l}{New Obj$\uparrow$} \\ \midrule
    % Ours (rand) & $1.73_{\pm 0.12}$  & $1.64_{\pm{0.21}}$ & $1.61_{\pm 0.07}$  & $1.72_{\pm{0.10}}$ \\
    Baseline(fs) & $59.78_{ \pm 5.75 } $ & $60.37_{ \pm 5.71 }$ & $64.76_{ \pm 1.26 } $ & $65.02_{ \pm 1.22 }$ \\
    Ours(full-fs) & $85.06_{ \pm 1.55 } $ & $85.17_{ \pm 1.47 }$ & $83.08_{ \pm 0.69 } $ & $83.70_{ \pm 0.88 }$ \\
    % Ours (SA) & $84.23_{\pm 3.93}$ & $84.04_{\pm 3.93}$ & $83.80_{\pm 0.83}$ & $83.43_{\pm 0.83}$ \\  \midrule % self attention 
    % \midrule
    \bottomrule
  \end{tabularx}
  \caption{
    Comparative results on the task success ratio
    for the baseline and \propmodel{} in reinforcement learning on stop condition.
    In stop condition, a submission action is not required and the goal object prediction is
    automatically sent to the oracle at the end of the dialogue.
}\label{tab:results_fs}
\end{centering}
\vspace{-1em}
\end{table}

% ask3_uniqer_rl_fs: $85.06_{ \pm 1.55 } $ & $85.17_{ \pm 1.47 }$ \\
% a3blfs: $59.78_{ \pm 5.75 } $ & $60.37_{ \pm 5.71 }$ \\
% ask4_uniqer_rl_fs: $83.08_{ \pm 0.69 } $ & $83.70_{ \pm 0.88 }$ \\
% a4blfs: $64.76_{ \pm 1.26 } $ & $65.02_{ \pm 1.22 }$ \\

\nibf{Additional Qualitative Samples (\S\redrb{6.3}).}
Extensive qualitative examples are presented in Fig.~\ref{fig:appendix_samples}.
From the samples, we can see that \propmodel{} made a full use of descriptive question
in all scenes, while \textit{Baseline} ended up with generating simple questions.
We also find that the question strategy of \textit{Baseline} was nearly fixed;
most of the time it was asking relative location question two times in the beginning
and simple material question at the end.
The results also reveal the \propmodel{}'s limitation.
It tend to ask extra questions to make its prediction perfect,
while the goal object is deemed to be found.
This suggests some improvements on answer submission are required in the future works.
Additionally, \propmodel{} fails when the goal
object is surrounded by too many identical objects.
In our future work, more complex referring expressions such as
``Is it second to the left of \textit{sth}?'' will be needed.

\subsection{Dataset Details (\S\redrb{3})}
\nibf{Statistics.}
% What is the data-size?
Both Ask3 and Ask4 datasets consist of  70K training, 7.5K validation, and 7.5K test images,
each of which includes three to ten objects.
The number of objects in Ask3 dataset is 455,216, 48,673, and 48,447,
for training, validation and test sets respectively,
while for Ask4 is 454,038, 48,317, and 48,674.
Ten questions per image are generated yielding 700K, 75K, and 75K questions
for training, validation, and test images, respectively.
Note that these questions are only used in supervised learning.
Additional statistics for the datasets are available as follows:
a distribution of the number of objects~Fig.~\ref{fig:obj_n_dist},
a distribution of the object attributes~Fig.~\ref{fig:obj_a_distrib},
and a distribution of the question attributes~Fig.~\ref{fig:q_distrib}.

\nibf{Scene Examples.}
Examples of scenes for both datasets are presented in Fig.~\ref{fig:scenes}.

\begin{figure*}[tbp] \begin{center}
  \includegraphics[width=\linewidth]{./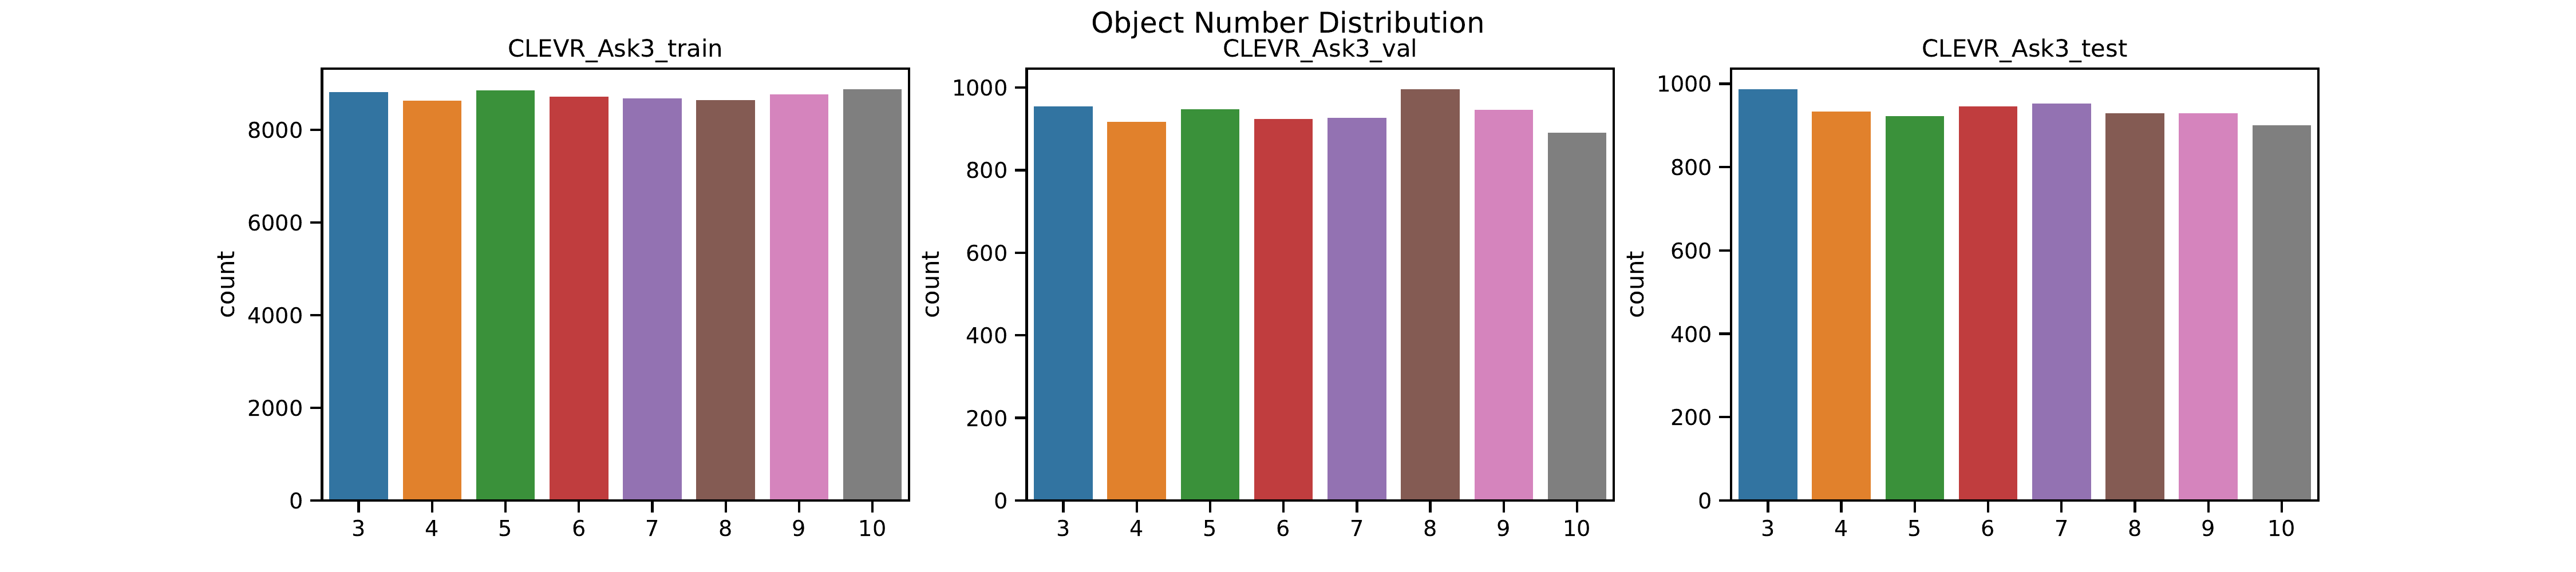}
  \includegraphics[width=\linewidth]{./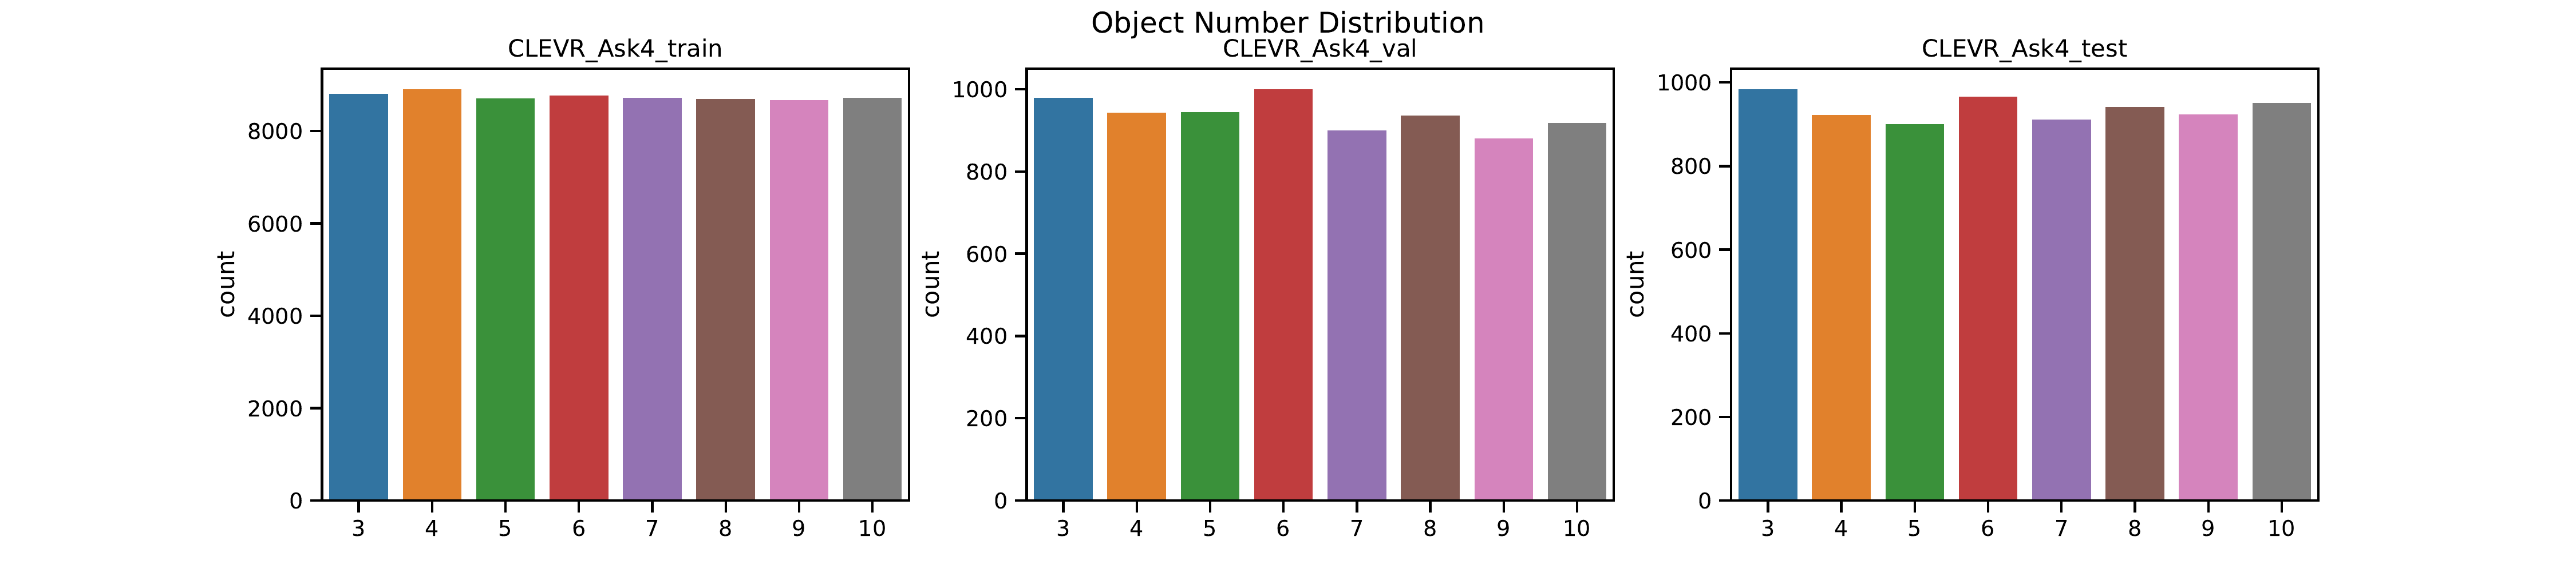}
  	\caption{
      Distribution of the number of objects in Ask3 and Ask4 dataset.
    }
    \label{fig:obj_n_dist}
  \end{center}
\vspace{-5mm}
\end{figure*}

\begin{figure*}[tbp] \begin{center}
  \includegraphics[width=.8\linewidth]{./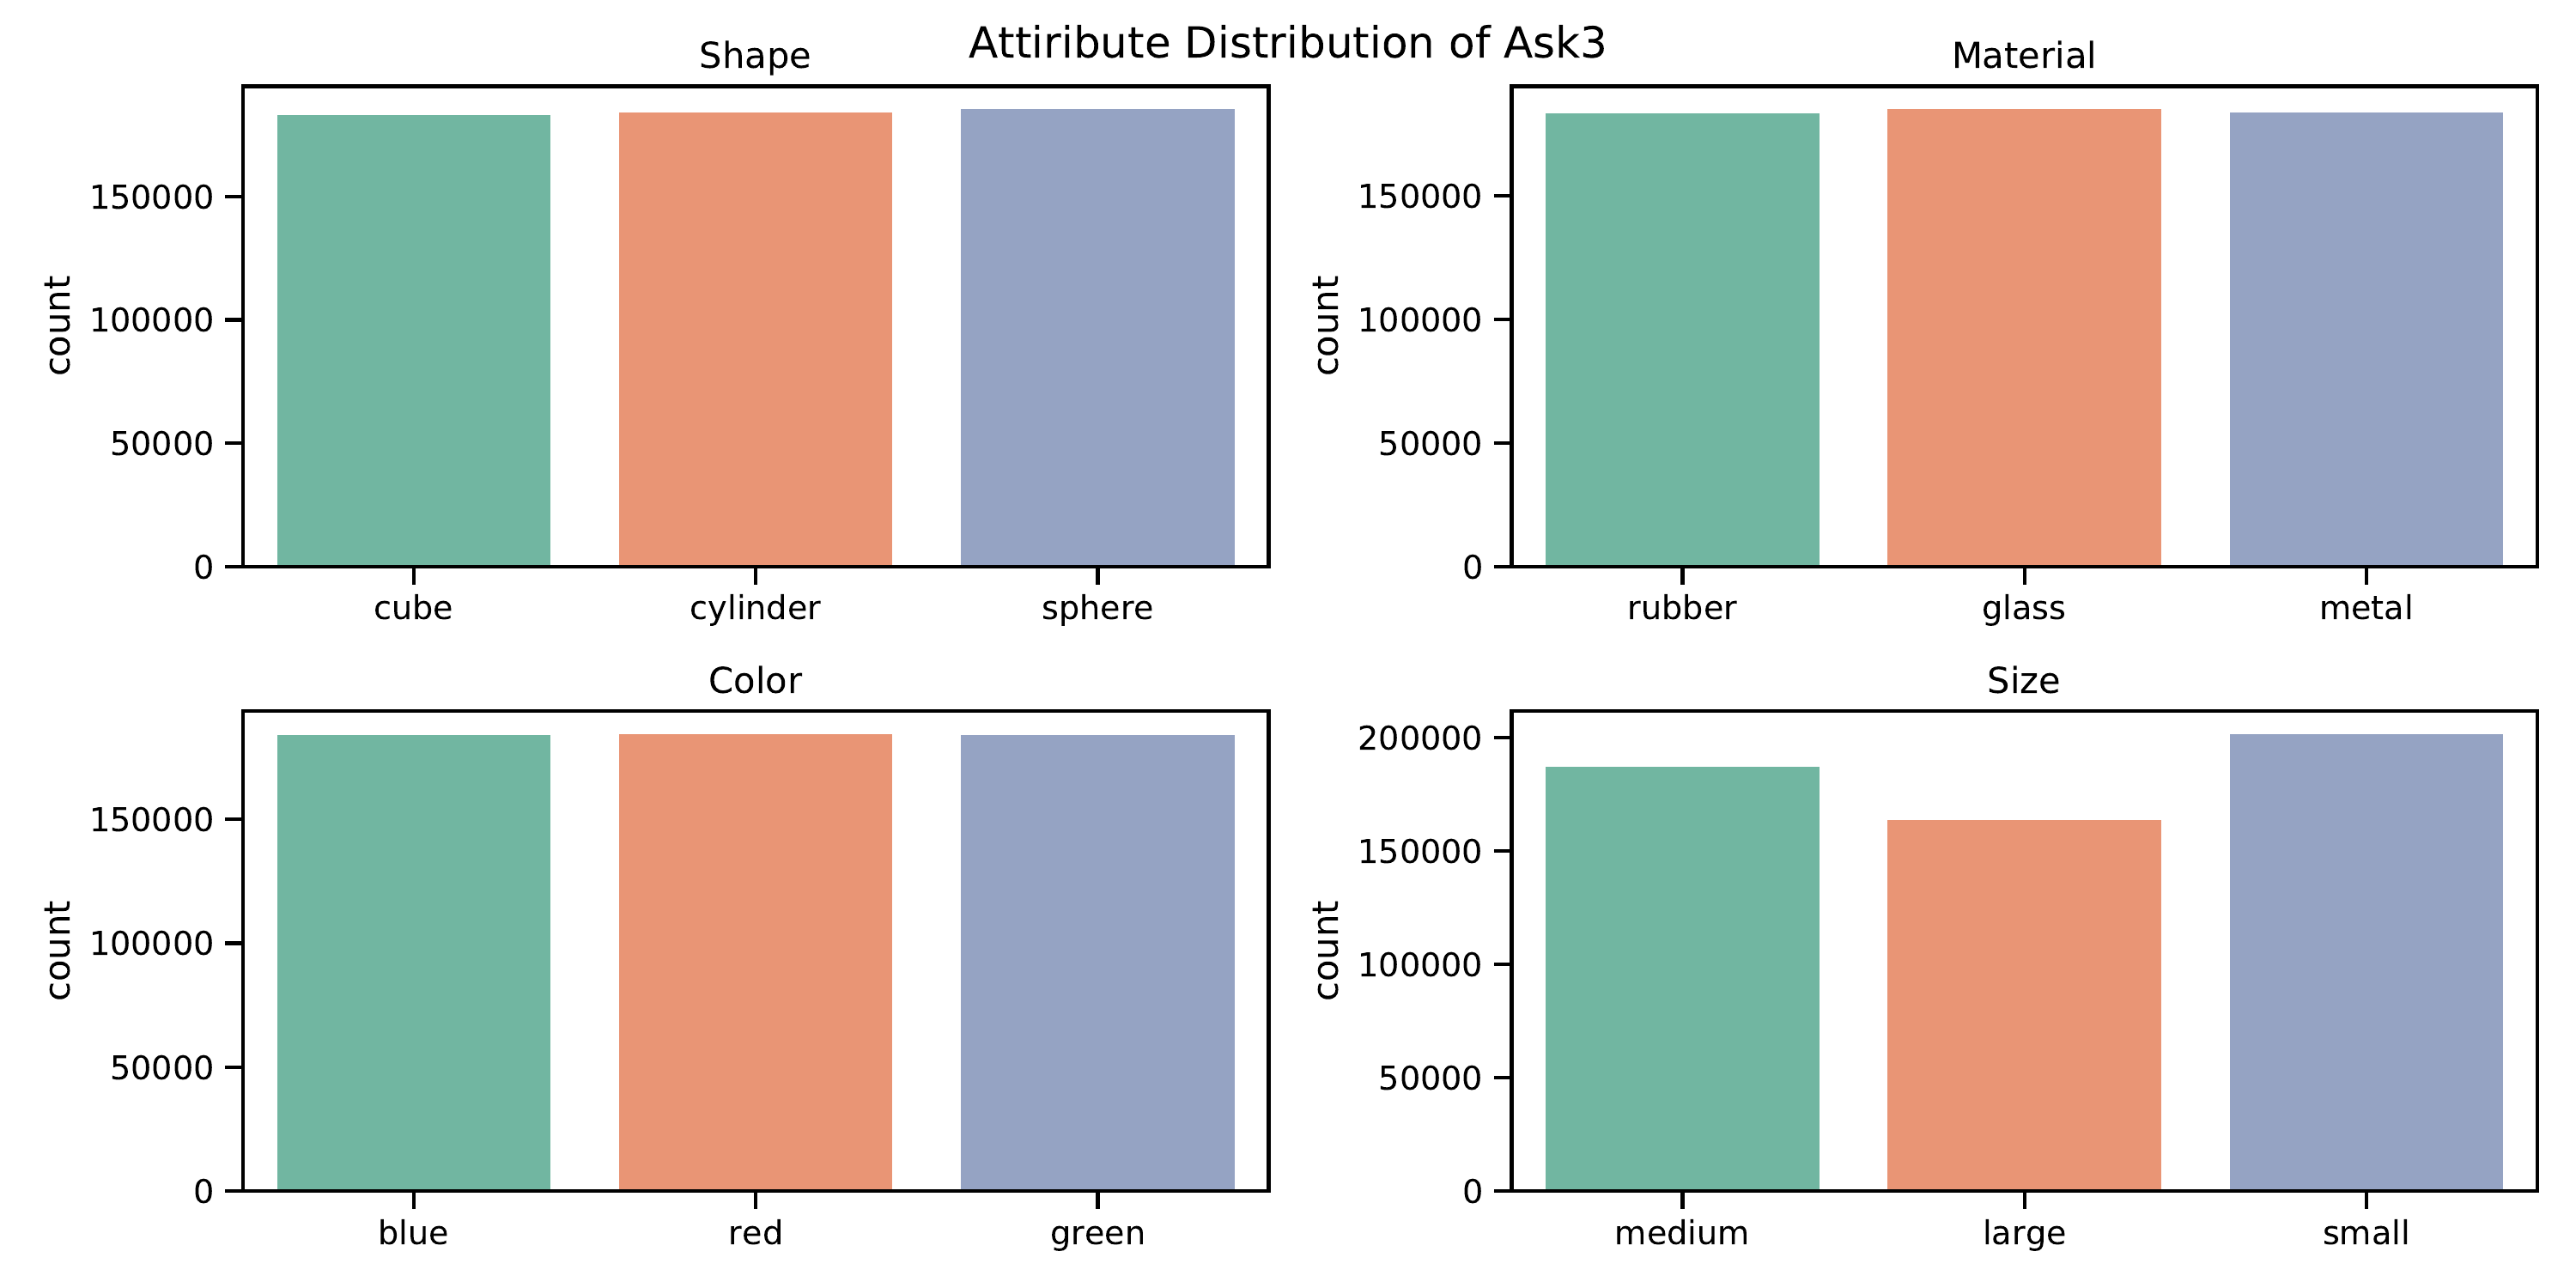}
  \includegraphics[width=.8\linewidth]{./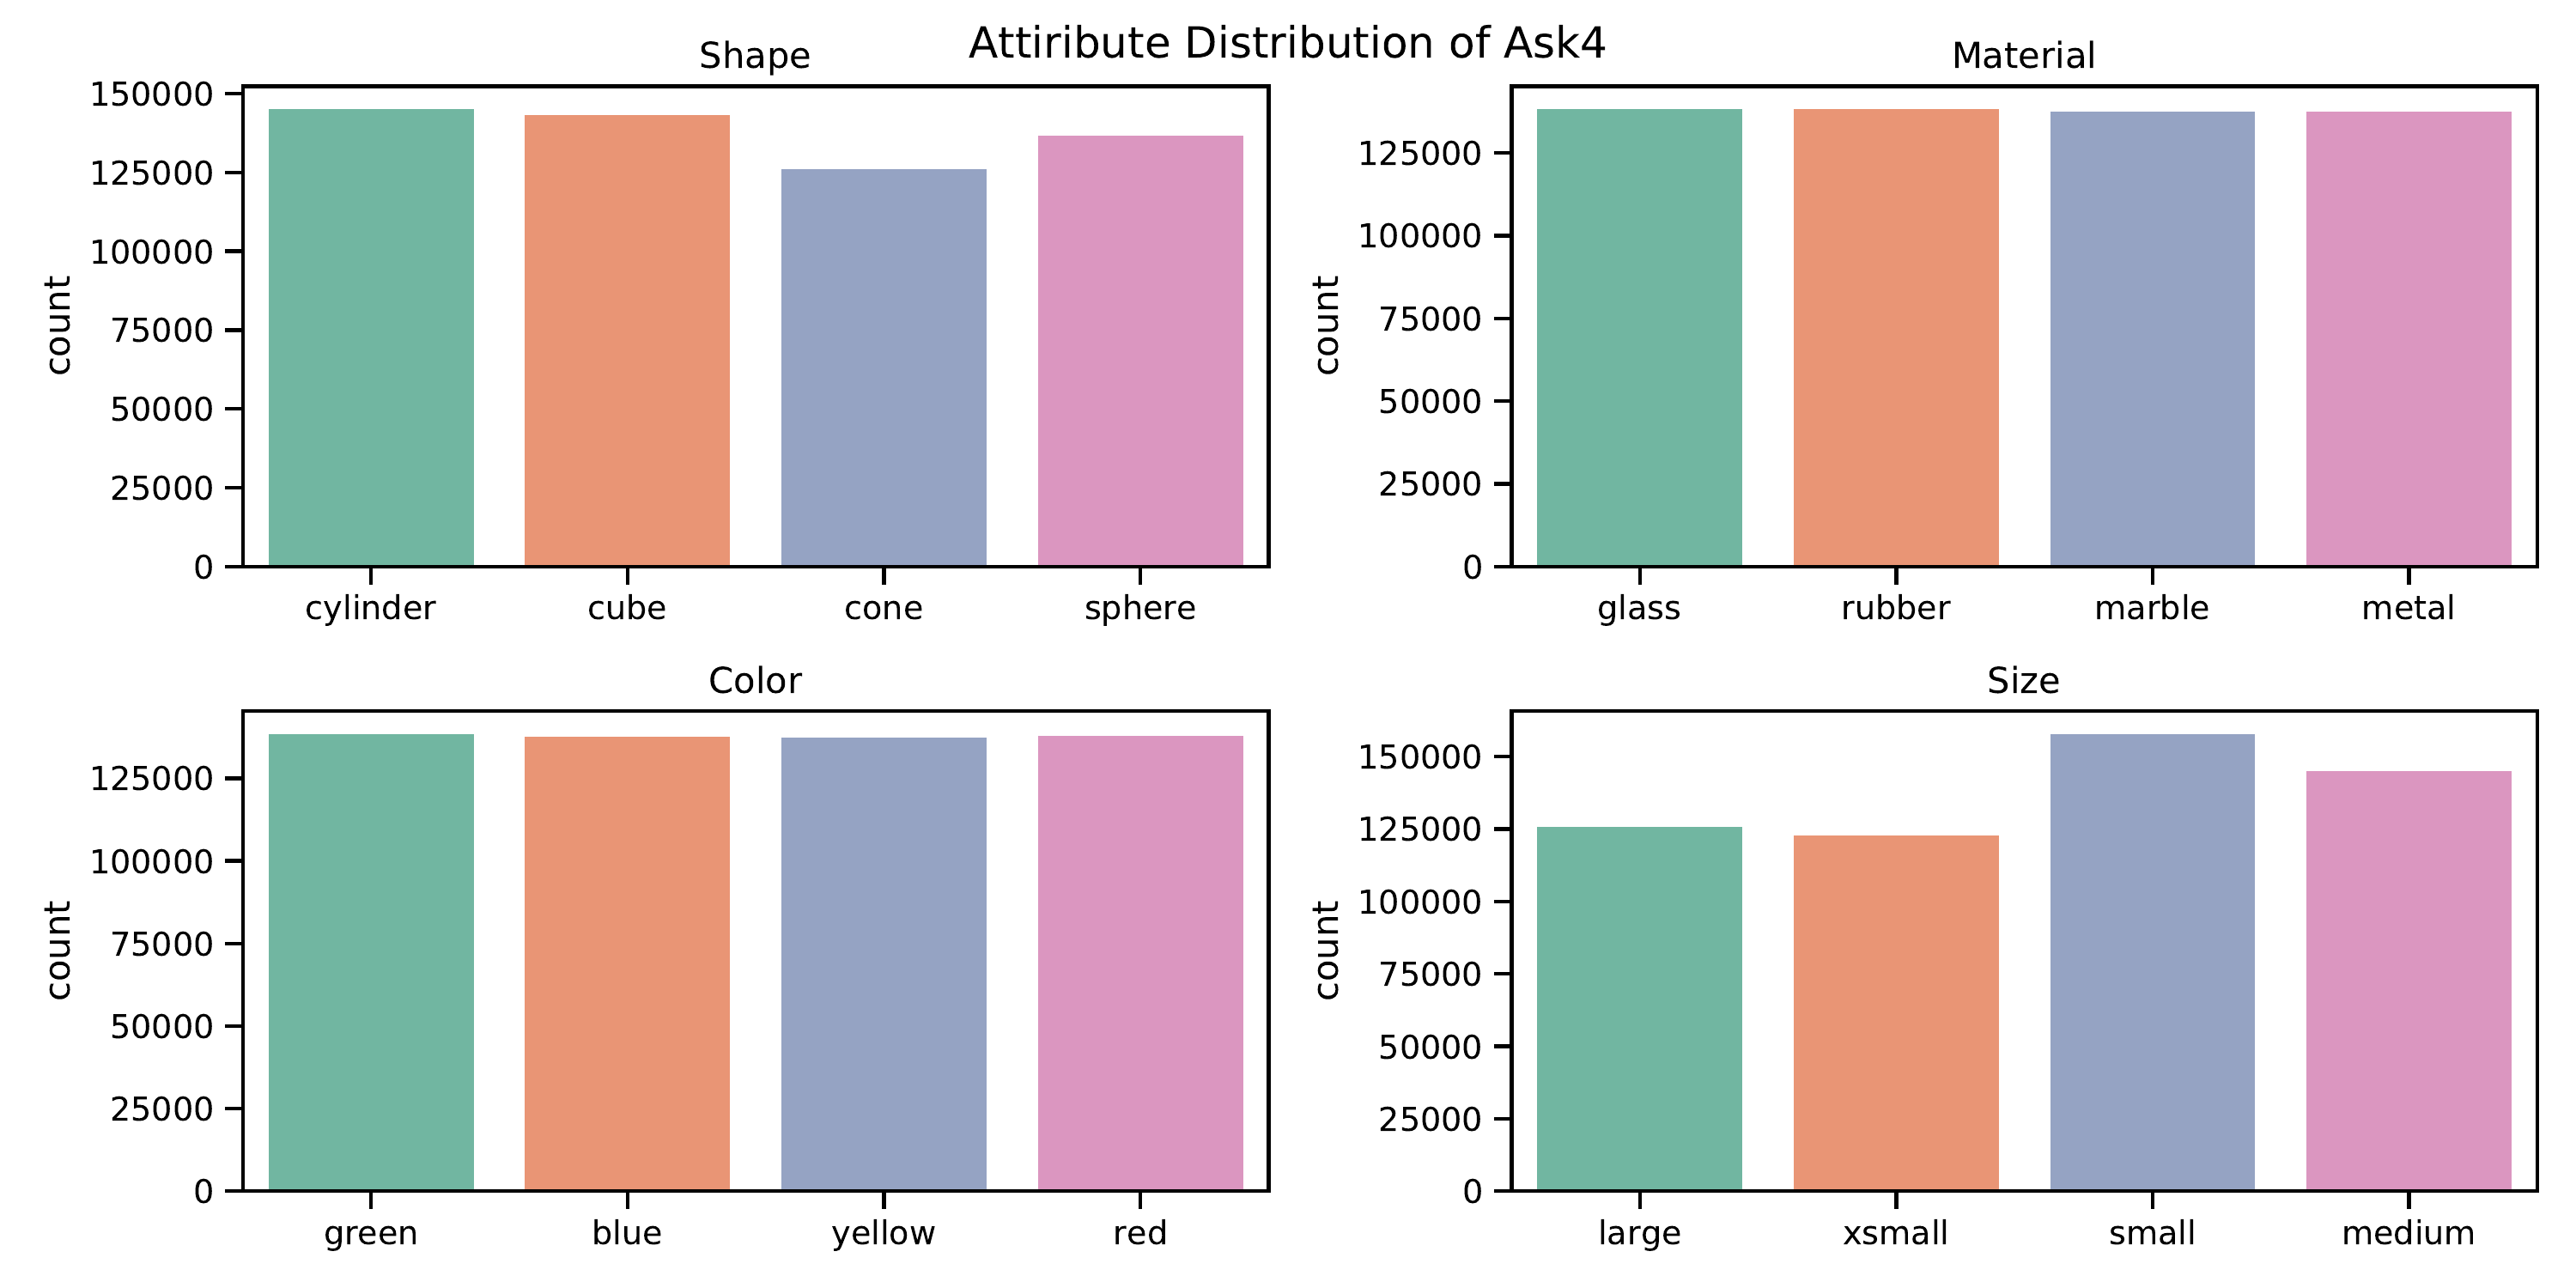}
  	\caption{
      Distribution of the attributes of objects in Ask3 and Ask4 dataset.
    }
    \label{fig:obj_a_distrib}
  \end{center}
\vspace{-5mm}
\end{figure*}

\begin{figure*}[tbp] \begin{center}
  \includegraphics[width=.45\linewidth]{./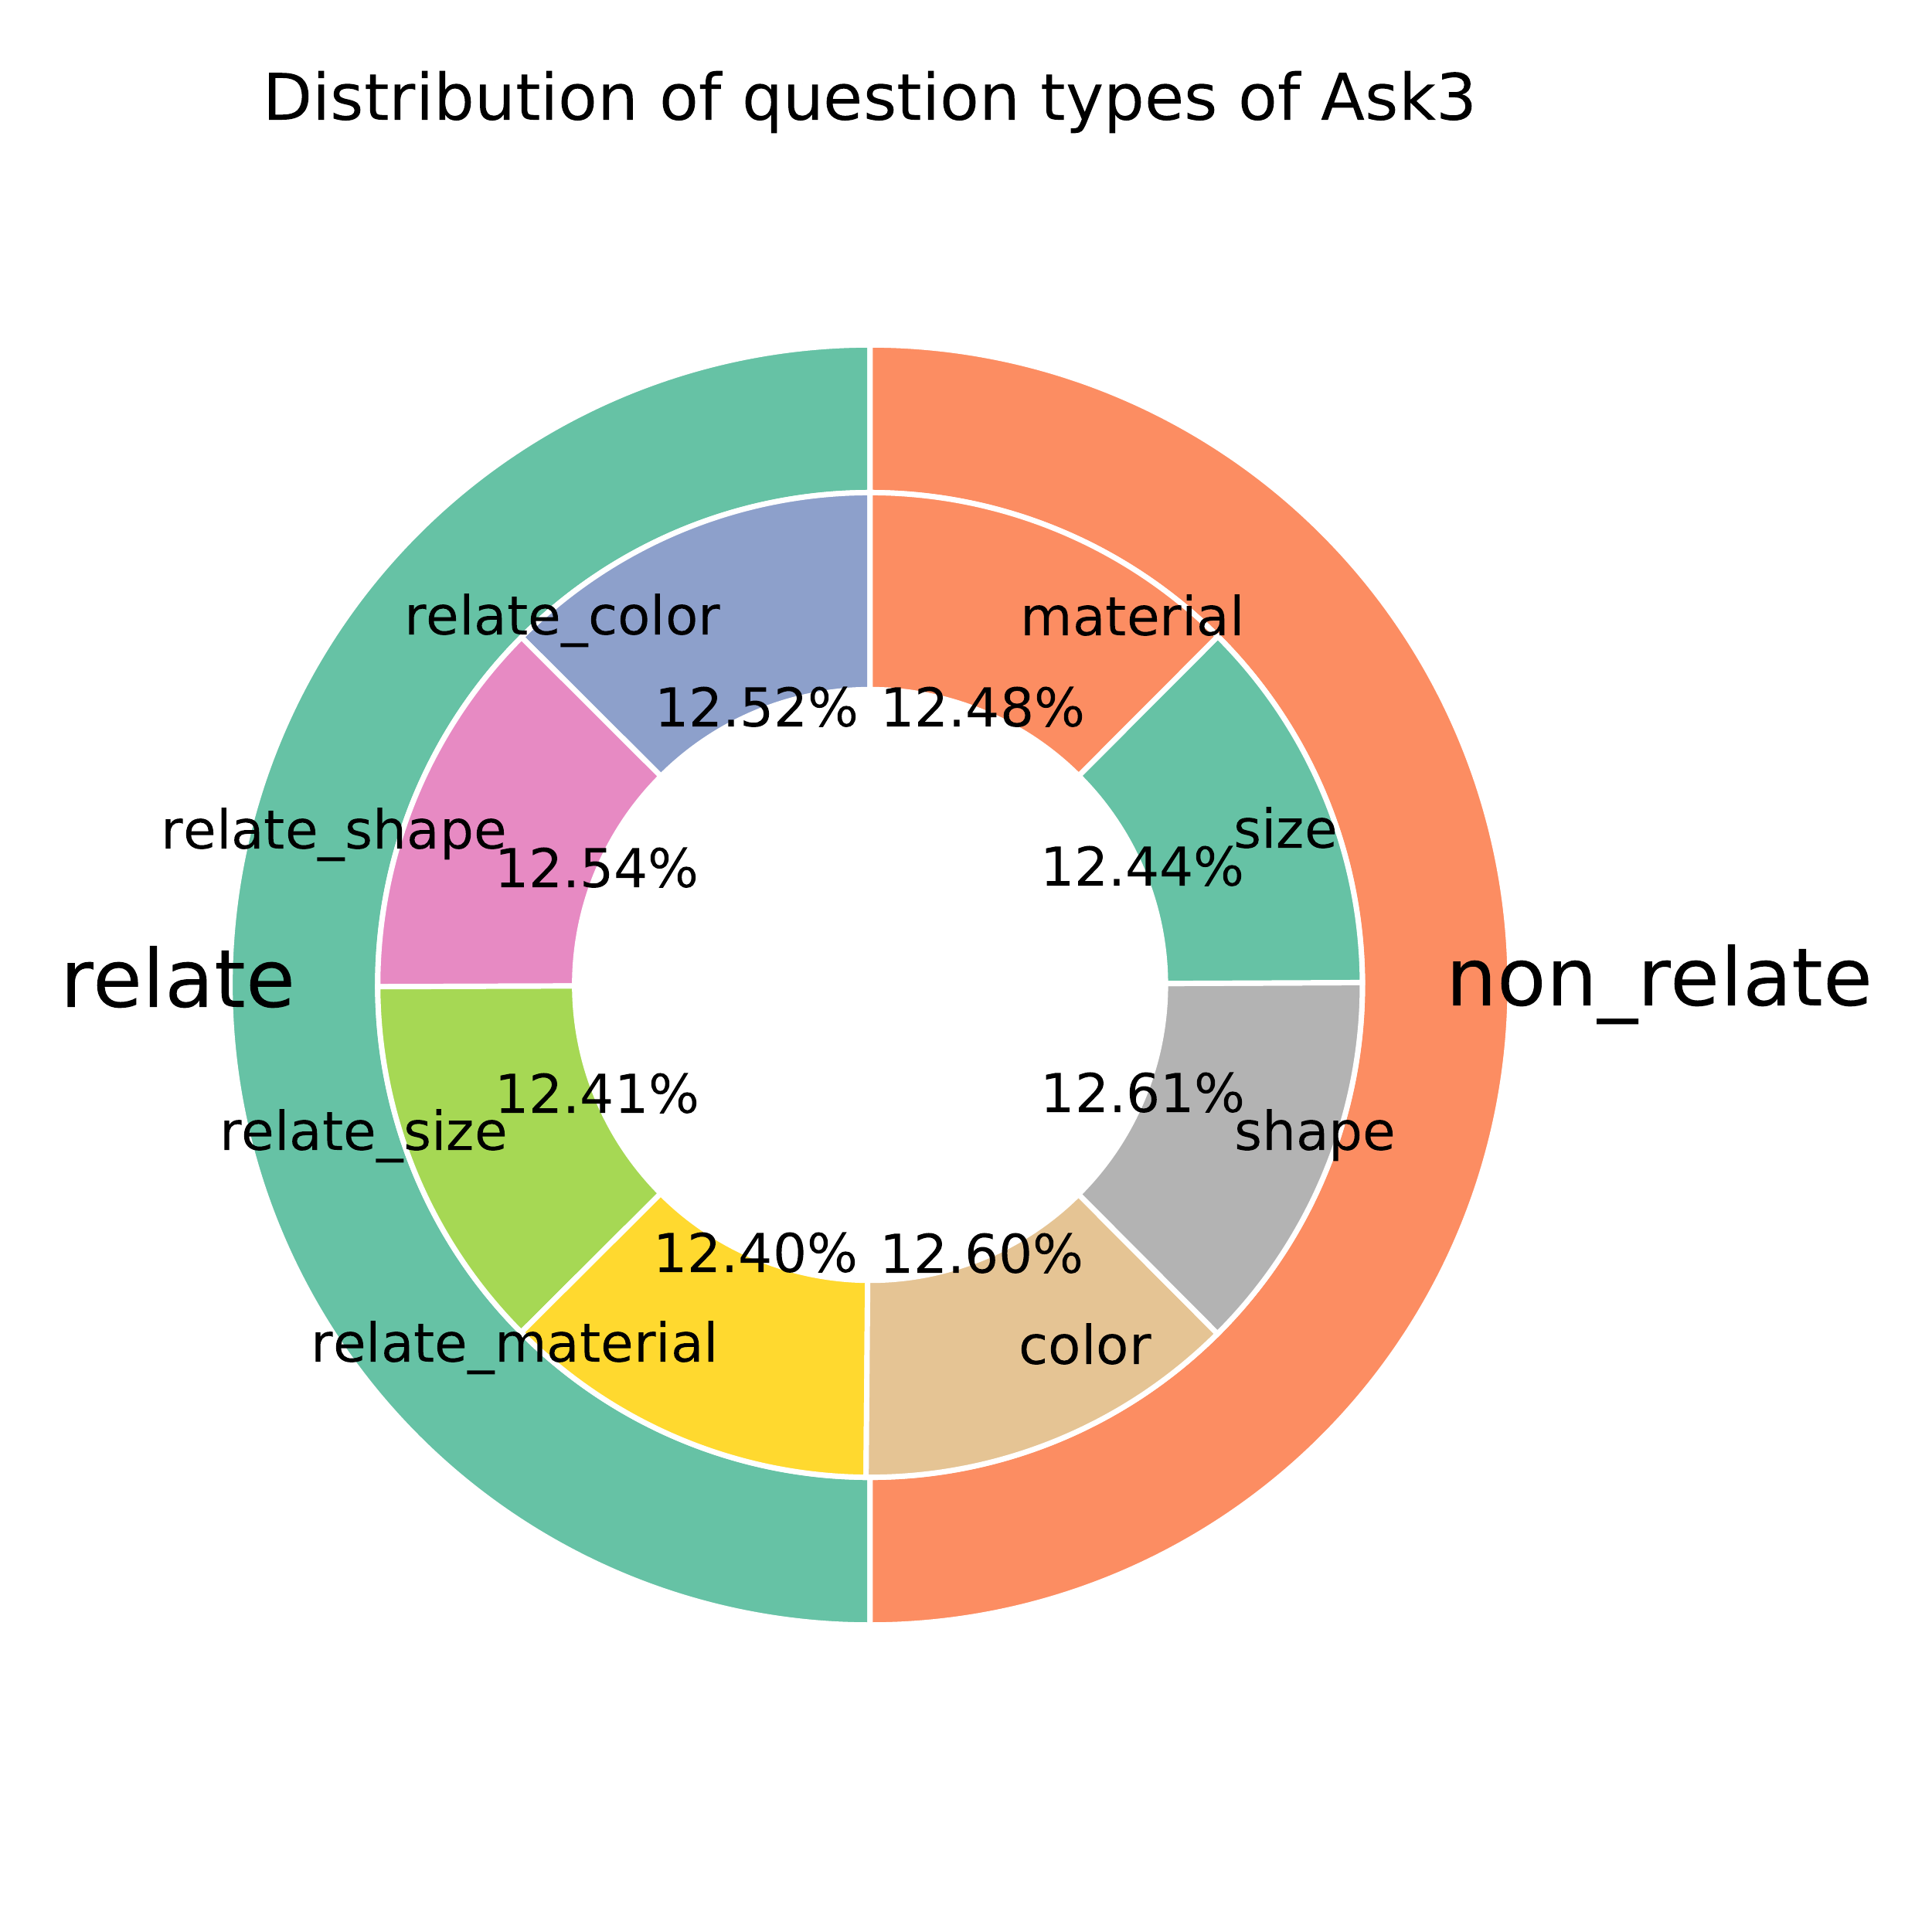}%
  \includegraphics[width=.45\linewidth]{./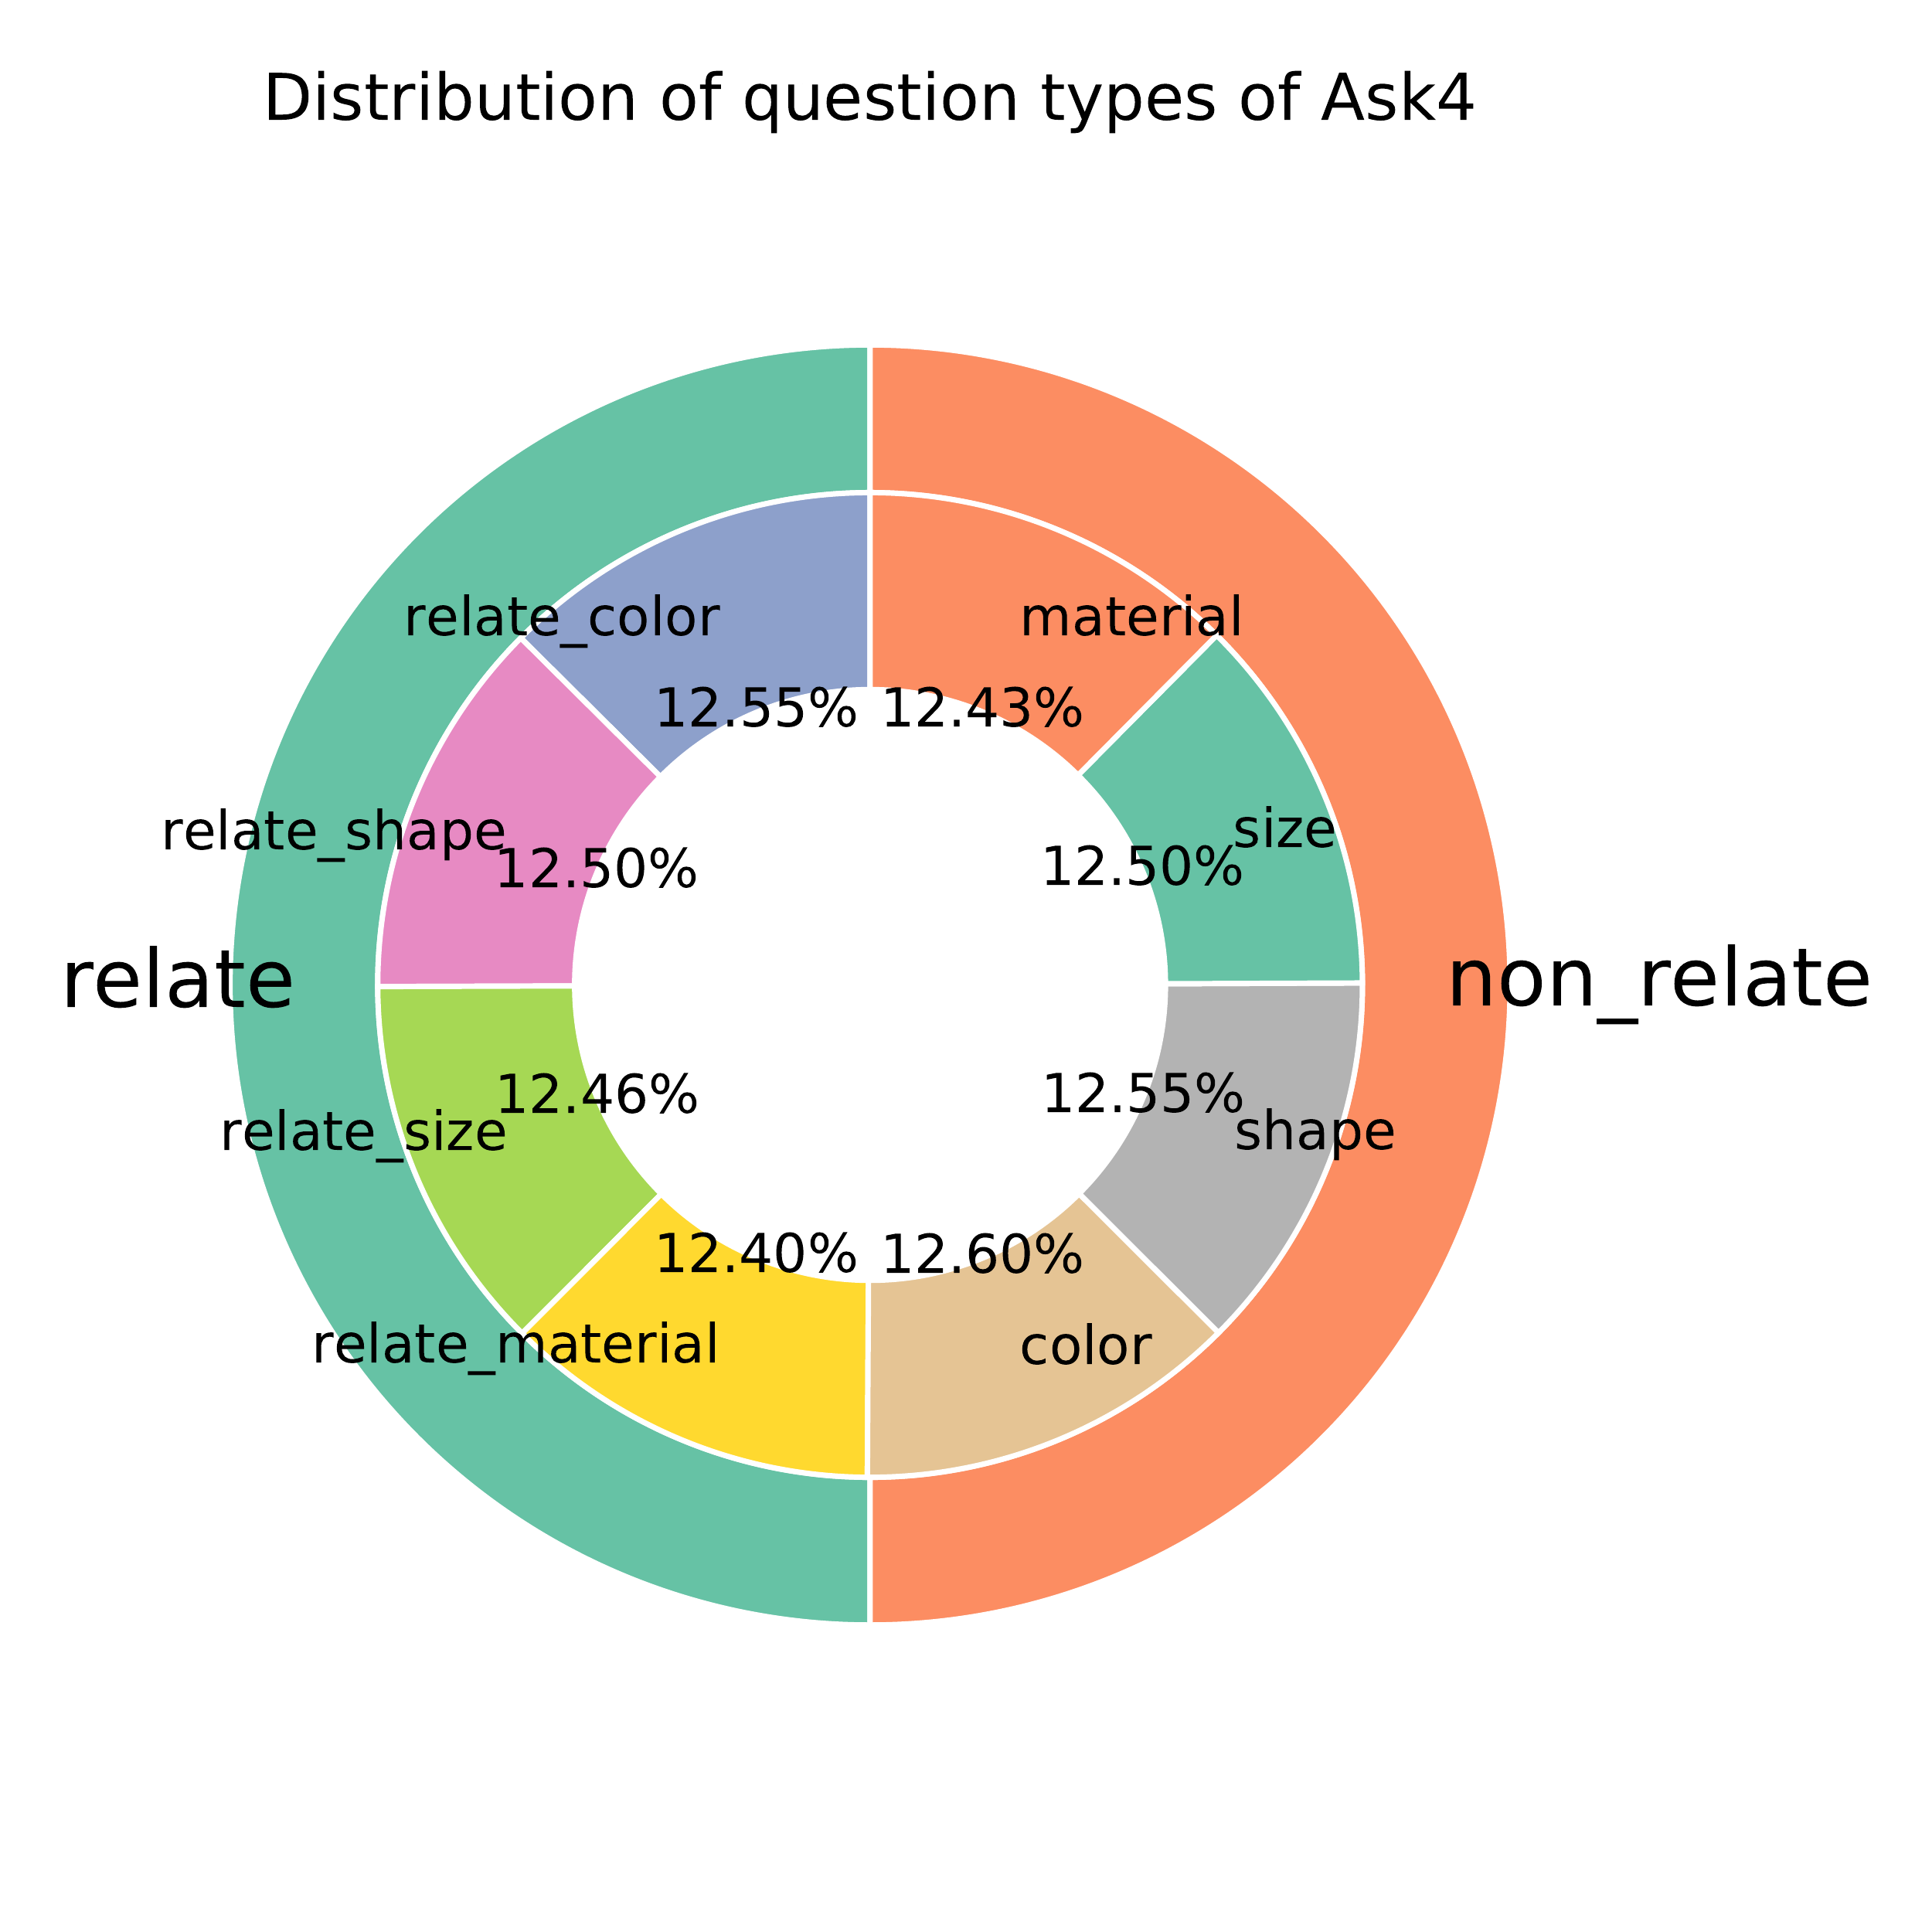}
  	\caption{
      Distribution of question attributes in Ask3 and Ask4 dataset.
    }
    \label{fig:q_distrib}
  \end{center}
\vspace{-5mm}
\end{figure*}

\begin{figure*}[tbp] \begin{center}
    \includegraphics[width=0.85\linewidth]{./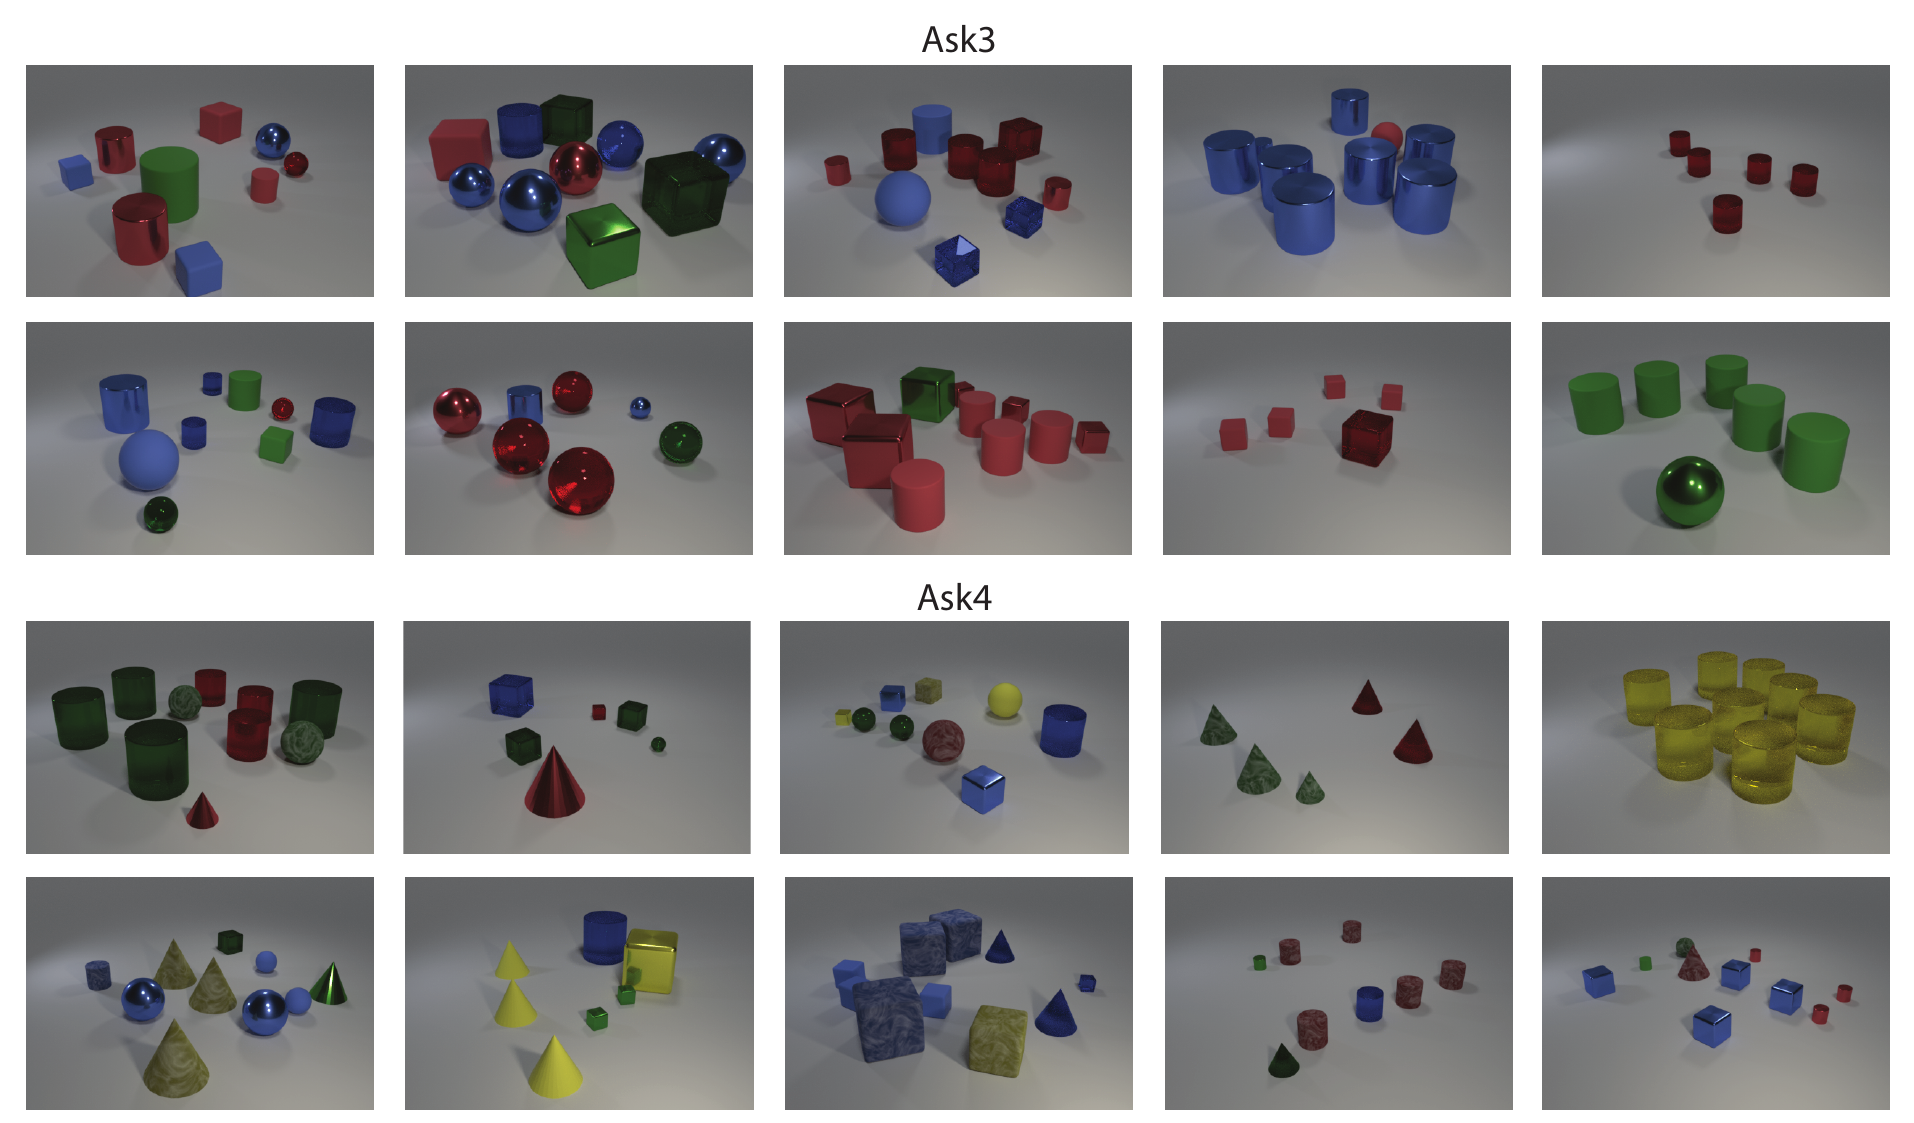}
  	\caption{
      Sample scenes in Ask3 and Ask4 dataset.
    }
    \label{fig:scenes}
  \end{center}
\vspace{-5mm}
\end{figure*}
